# Supplementary material for: A Consumer-Theoretic Characterization of Fisher Market Equilibria
Source: arXiv:2107.08153 source file (2022-01-04)
Supplement: Supplementary file 1 [file proofs_sec6.tex]

We first prove that by setting $\gamma$ to be 5 times the maximum demand for any good throughout the 
entropic t\^atonnement process
% algorithm for the t\^atonnement rule given in \Crefrange{tatonnement-KL}{tatonnement-KL2}
, we can bound the change in the prices of goods in each round. We will use the fact that the change in the price of each good is bounded as an assumption in most of the following results.

\begin{lemma}
\label{price-change}
Suppose that entropic t\^atonnement process 
% given in \Cref{tatonnement-KL} and \Cref{tatonnement-KL2} 
is run with $\gamma = 5 \max\limits_{\substack{t \in \N\\ \good \in \goods}} \{\demand[\good]^t\}$, then the following holds for all $t \in \N$:
\begin{align*}
    e^{-\frac{1}{5}} \price[\good]^{t}\leq \price[\good]^{t+1} \leq e^{\frac{1}{5}} \price[\good]^{t} \text{ and }\frac{|\pricediff[\good]|}{\price[\good]} \leq \frac{1}{4}
\end{align*}
\end{lemma}
 
\begin{proof}[\Cref{price-change}]
The price of of a good can at most increase by a factor of $e^{\frac{1}{5}}$:
\begin{align*}
    \price[\good]^{t+1} &= \price[\good]^t \exp\left\{\frac{\excess[\good](\price^t)}{5 \max\limits_{\substack{t \in \N\\ \good \in \goods}} \{\demand[\good]^t\}}\right\} = \price[\good]^t \exp\left\{\frac{\demand[\good]^t - 1}{5 \max\limits_{\substack{t \in \N\\ \good \in \goods}} \{\demand[\good]^t\}}\right\} \leq \price[\good]^t \exp\left\{\frac{\demand[\good]^t}{5 \max\limits_{\substack{t \in \N\\ \good \in \goods}} \{\demand[\good]^t\}}\right\}    % &\leq \price[\good]^t \exp\left\{ \frac{\max\limits_{\substack{t \in \N\\ \good \in \goods}} \{ \demand[\good]^t \}}{5 \max\limits_{\substack{t \in \N\\ \good \in \goods}} \{\demand[\good]^t\}}\right\}\\
    =\price[\good]^t e^{\frac{1}{5}}
\end{align*}
and decrease by a factor of $e^{-\frac{1}{5}}$:
\begin{align*}
    \price[\good]^{t+1} &= \price[\good]^t \exp\left\{\frac{\excess[\good](\price^t)}{5 \max\limits_{\substack{t \in \N\\ \good \in \goods}} \{\demand[\good]^t\}}\right\} = \price[\good]^t \exp\left\{\frac{\demand[\good]^t - 1}{5 \max\limits_{\substack{t \in \N\\ \good \in \goods}} \{\demand[\good]^t\}}\right\} \geq \price[\good]^t \exp\left\{\frac{-1}{5 \max\limits_{\substack{t \in \N \good \in \goods}} \{\demand[\good]^t\}}\right\} =\price[\good]^t e^{-\frac{1}{5}}
\end{align*}

Hence, we have $e^{-\frac{1}{5}} \price[\good]^{t}\leq \price[\good]^{t+1} \leq e^{\frac{1}{5}} \price[\good]^{t}$. substracting $\price[\good]^t$ from both sides and dividing by $\price[\good]^t$, we obtain:
\begin{align*}
    \frac{|\pricediff[\good]|}{\price[\good]^t} = \frac{|\price[\good]^{t+1} - \price[\good]^{t}|}{\price[\good]^t} \leq e^{\nicefrac{1}{5}} - 1 \leq \frac{1}{4} 
\end{align*}
\end{proof}

The following two results are due to \citeauthor{fisher-tatonnement} \cite{fisher-tatonnement}. We include their proofs for completeness.

\begin{lemma}{\cite{fisher-tatonnement}}\label{leontief-ineq}
For all $\good \in \goods$:
\begin{align*}
    \frac{1}{\budget[\buyer] } \sum_{\good \in \goods} \sum_{k \in \goods} \demand[\buyer][\good]^t\demand[\buyer][k]^t|\pricediff[\good]||\pricediff[k]| \leq \sum_{l \in \goods} \frac{\demand[\buyer][l]^t}{\price[l]^t}(\pricediff[l])^2
\end{align*}
\end{lemma}

\begin{proof}[\Cref{leontief-ineq}]
First, note that by Walras' law we have $\budget[\buyer] = \sum_{k \in \goods} \demand[\buyer][k]^t \price[k]^t$;
\begin{align*}
    \budget[\buyer]\sum_{l \in \goods} \frac{\demand[\buyer][l]^t}{\price[l]^t}(\pricediff[l])^2 &= \sum_{l \in \goods} \frac{\left(\sum_{k \in \goods} \demand[\buyer][k]^t \price[k]^t \right)\demand[\buyer][l]^t}{\price[l]^t}(\pricediff[l])^2\\
    &=\sum_{l \in \goods} \sum_{k \in \goods} \demand[\buyer][l]^t \demand[\buyer][k]^t \frac{\price[k]^t}{\price[l]^t} (\pricediff[l])^2\\
    &= \sum_{l \in \goods} (\demand[\buyer][l]^t)^2 (\pricediff[l])^2 + \sum_{l \in \goods} \sum_{k \neq l } \demand[\buyer][l]^t \demand[\buyer][k]^t \frac{\price[k]^t}{\price[l]^t} (\pricediff[l])^2\\
    &= \sum_{l \in \goods} (\demand[\buyer][l]^t)^2 (\pricediff[l])^2 + \sum_{k \in \goods} \sum_{k \leq l} \demand[\buyer][k]^t \demand[\buyer][l]^t \left( \frac{\price[k]^t}{\price[l]^t} (\pricediff[l])^2 + \frac{\price[l]^t}{\price[k]^t} \ (\pricediff[k])^2\right)
\end{align*}

Now, we apply the AM-GM inequality: 
\begin{align*}
\budget[\buyer] \sum_{l \in \goods} \frac{\demand[\buyer][l]^t}{\price[l]^t} (\pricediff[l])^2 &\geq \sum_{l \in \goods} (\demand[\buyer][l]^t)^2 (\pricediff[l])^2 + \sum_{k < l} \demand[\buyer][k]^t \demand[\buyer][l]^t\left(2 |\pricediff[l]||\pricediff[k]||\right)\\
&= \sum_{\good \in \goods} \sum_{k \in \goods} \demand[\buyer][\good]^t \demand[\buyer][k]^t |\pricediff[\good]||\pricediff[k]|
\end{align*}
\end{proof}

\begin{lemma}\cite{fisher-tatonnement} \label{kl-divergence-1}
Suppose that for all $\good \in \goods$, $\frac{|\pricediff[\good]|}{\price[\good]^t} \leq \frac{1}{4}$, then:
\begin{align}
    \frac{(\pricediff[\good])^2}{\price[\good]^t} \leq \frac{9}{2} \divergence[\mathrm{KL}][{\price[\good]^t + \pricediff[\good]}][{\price[\good]^t}]
\end{align}
\end{lemma}

\begin{proof}[\Cref{kl-divergence-1}]
The bound $\log(x) \geq x - \frac{11}{18}x^2$ for $|x|\frac{1}{4}$ is used below:
\begin{align*}
    \divergence[\mathrm{KL}][{\price[\good]^t + \pricediff[\good]}][{\price[\good]^t}] &= (\price[\good]^t + \pricediff[\good])(\log(\price[\good]^t + \pricediff[\good])) - ( \price[\good]^t + \pricediff[\good] - \price[\good]^t\log(\price[\good]) + \price[\good]^t - \log(\price[\good]^t) \pricediff[\good]\\
    &= - \pricediff[\good] + (\price[\good]^t + \pricediff[\good]) \log \left(1 + \frac{\pricediff[\good]}{\price[\good]^t}\right)\\
    &\geq - \pricediff[\good] + (\price[\good]^t + \pricediff[\good]) \log \left( \frac{\pricediff[\good]}{\price[\good]^t} - \frac{11}{18} \frac{(\pricediff[\good])^2}{(\price[\good]^t)^2} \right)\\
    &\geq \frac{7}{18} \frac{(\pricediff[\good])^2}{\price[\good]^t} \left( 1 - \frac{11}{7} \frac{\pricediff[\good]}{\price[\good]^t}\right)\\
    &= \frac{7}{18} \frac{17}{28} \frac{(\pricediff[\good])^2}{\price[\good]^t}\\
    &\geq \frac{2}{9} \frac{(\pricediff[\good])^2}{\price[\good]^t}
\end{align*}
\end{proof}

The following lemma allows us to relate the change in prices to the KL-divergence.

An important result in microeconomics is the \mydef{law of demand} which states that when the price of a good increases, the Hicksian demand for that good decreases in a very general setting of utility functions \cite{levin-notes, mas-colell}. We state a weaker version of the law of demand which is re-formulated to fit the t\^atonnement framework.

\begin{lemma}[Law of Demand]\cite{levin-notes,mas-colell}\label{law-of-demand}
Suppose that $\forall \good \in \goods, t \in \N, \price[\good]^t, \price[\good]^{t+1} \geq 0$ and $\util[\buyer]$ is continuous and concave. Then, $\sum_{\good \in \goods} \pricediff[\good] \left(\hicksian[\buyer][\good]^{t+1} - \hicksian[\buyer][\good]^{t}\right) \leq 0$.
\end{lemma}

A simple corollary of the law of demand which is used throughout the rest of this paper is that, during t\^atonnement, the change in expenditure of the next time period is always less than or equal to the change in expenditure of the previous time period's.

\begin{corollary}\label{law-of-demand-corollary}
Suppose that $\forall t \in \N, \good \in \goods, \price[\good]^t,  \price[\good]^{t+1} \geq 0$ and $\util[\buyer]$ is continuous and concave then $\forall t \in \N, \sum_{\good \in \goods} \pricediff[\good] \hicksian[\buyer][\good]^{t+1}  \leq \sum_{\good \in \goods} \pricediff[\good] \hicksian[\buyer][\good]^{t}$.
\end{corollary} 

The following lemma simply restates an essential fact about expenditure functions and Hicksian demand, namely that the Hicksian demand is the minimizer of the expenditure function.

\begin{lemma}\label{hicksian-is-expend-minimizer}
Suppose that $\forall \good \in \goods, \price[\good]^t, t \in \N \hicksian[\buyer][\good]^t, \hicksian[\buyer][\good]^{t+1} \geq 0$ and $\util[\buyer]$ is continuous and concave then $\sum_{\good \in \goods} \hicksian[\buyer][\good]^t \price[\good]^t \leq \sum_{\good \in \goods} \hicksian[\buyer][\good]^{t+1} \price[\good]^{t}$.
\end{lemma}

\begin{proof}[\Cref{hicksian-is-expend-minimizer}]
For the sake of contradiction, assume that $\sum_{\good \in \goods} \hicksian[\buyer][\good]^t \price[\good]^t > \sum_{\good \in \goods} \hicksian[\buyer][\good]^{t+1} \price[\good]^{t}$. By the definition of the Hicksian demand, we know that the bundle $\hicksian[\buyer]^t$ provides the buyer with one unit of utility. 
Recall that the expenditure at any price $\price$ is equal to the sum of the product of the Hicksian demands and prices, that is $\expend[\buyer](\price, 1) = \sum_{\good \in \goods} \hicksian[\buyer][\good](\price, 1) \price[\good]$. Hence, we have $\expend[\buyer](\price[\good]^t, 1) = \sum_{\good \in \goods} \hicksian[\buyer][\good]^t \price[\good]^t > \sum_{\good \in \goods} \hicksian[\buyer][\good]^{t+1} \price[\good]^{t} = \expend[\buyer](\price^t, 1)$, a contradiction.
\end{proof}

The following lemma in conjunction with \Cref{law-of-demand-corollary} and \Cref{hicksian-is-expend-minimizer} are key in proving that \Cref{ineq-devanur} holds allowing us to establish convergence of t\^atonnement in a general setting of utility functions.
Additionally, the lemma relates the Marshallian demand of homogeneous utility functions to their Hicksian demand by taking advantage of \Cref{homo-expend}. 

\begin{lemma}\label{equiv-def-demand}
Suppose that $\util[\buyer]$ is CSCH, then the following holds:
\begin{align*}
    &\forall \good \in \goods &\marshallian[\buyer][\good](\price, \budget[\buyer]) = \frac{\budget[\buyer] \hicksian[\buyer][\good](\price, 1)}{\sum_{\good \in \goods} \hicksian[\buyer][\good](\price, 1) \price[\good]}
\end{align*}
\end{lemma}

\begin{proof}[\Cref{equiv-def-demand}]
We note that when utility function $\util[\buyer]$ is strictly concave, the Marshallian and Hicksian demand are unique making the following equalities well-defined.
\begin{align*}
    \frac{\budget[\buyer] \hicksian[\buyer][\good](\price, 1)}{\sum_{\good \in \goods} \hicksian[\buyer][\good](\price, 1) \price[\good]} &= \frac{\budget[\buyer] \hicksian[\buyer][\good](\price, 1)}{\expend[\buyer](\price, 1)} && \text{(Definition of expenditure function)}\\
    &= \budget[\buyer]\indirectutil[\buyer](\price, 1) \hicksian[\buyer][\good](\price, 1) && \text{(\Cref{inverse-expend})}\\
    &= \indirectutil[\buyer](\price, \budget[\buyer]) \hicksian[\buyer][\good](\price, 1) && \text{(\Cref{homo-indirect-util})}\\
    &= \hicksian[\buyer][\good](\price, \indirectutil[\buyer](\price, \budget[\buyer])) && \text{(\Cref{homo-expend})}\\
    &= \marshallian[\buyer][\good](\price, \budget[\buyer]) && \text{(Marshallian Demand Identity \Cref{hicksian-marshallian})}
\end{align*}
\end{proof}

% \newgeometry{left=7mm, right=7mm}

\begin{lemma}\label{fix-buyer-bound}
Suppose that $\frac{|\pricediff[\good]|}{\price[\good]^t} \leq \frac{1}{4}$, then
\begin{align*}
    &\budget[\buyer] \log \left( 1 - \frac{\sum_{\good \in \goods} \hicksian[\buyer][\good]^{t+1} \pricediff[\good]}{\sum_{\good \in \goods} \hicksian[\buyer][\good]^{t+1} \price[\good]^t} \left( 1 + \frac{\sum_{\good \in \goods} \hicksian[\buyer][\good]^{t+1} \pricediff[\good]}{\sum_{\good \in \goods} \hicksian[\buyer][\good]^{t+1} \price[\good]}\right)^{-1}  \right)
    \leq \frac{4}{3} \sum_{\good \in \goods} \demand[\buyer][\good]^t \left( \frac{(\pricediff[\good])^2}{\price[\good]^t} \right) - \sum_{\good \in \goods} \pricediff[\good] \left( \frac{ \budget[\buyer] \hicksian[\buyer][\good]^{t+1} }{\sum_{\good \in \goods} \hicksian[\buyer][\good]^{t+1} \price[\good]^t} \right)
\end{align*}
\end{lemma}

\begin{proof}[\Cref{fix-buyer-bound}]
First, we note that $\sum_{\good \in \goods} \hicksian[\buyer][\good]^{t+1} \price[\good]^t > 0$ because prices during our t\^atonnement rule reach 0 only asymptotically; and likewise, prices reach $\infty$ only asymptotically, which implies that Hicksian demand is always strictly positive. This fact will come handy, as we divide some expressions by  $\sum_{\good \in \goods} \hicksian[\buyer][\good]^{t+1} \price[\good]^t$.

Fix $t$ and $\buyer$.
Since by our assumptions $|\pricediff[\good]| \leq \frac{\price[\good]^t}{4}$, we have $0 \leq \frac{|\sum_{\good \in \goods} \hicksian[\buyer][\good]^{t+1} \pricediff[\good]|}{\sum_{\good \in \goods} \hicksian[\buyer][\good]^{t+1} \price[\good]^t} \leq \frac{1}{4}\frac{\sum_{\good \in \goods} \hicksian[\buyer][\good]^{t+1} \price[\good]^t}{\sum_{\good \in \goods} \hicksian[\buyer][\good]^{t+1} \price[\good]^t} \leq \frac{1}{4}$.
We can then use the bound $1-x(1+x)^{-1} \leq 1 + \frac{4}{3} x^2 - x$, for $0 \leq |x| \leq \frac{1}{4}$, with $x = \frac{\sum_{\good \in \goods} \hicksian[\buyer][\good]^{t+1} \pricediff[\good]}{\sum_{\good \in \goods} \hicksian[\buyer][\good]^{t+1} \price[\good]^t}$, to get:
\begin{align*}
    \budget[\buyer] \log \left(1 - \frac{\sum_{\good \in \goods} \hicksian[\buyer][\good]^{t+1} \pricediff[\good]}{\sum_{\good \in \goods} \hicksian[\buyer][\good]^{t+1} \price[\good]^t} \left( 1 + \frac{\sum_{\good \in \goods} \hicksian[\buyer][\good]^{t+1} \pricediff[\good]}{\sum_{\good \in \goods} \hicksian[\buyer][\good]^{t+1} \price[\good]}\right)^{-1}  \right)\\
    \leq \budget[\buyer] \log \left( 1 + \frac{4}{3}\left( \frac{\sum_{\good \in \goods} \hicksian[\buyer][\good]^{t+1} \pricediff[\good]}{\sum_{\good \in \goods} \hicksian[\buyer][\good]^{t+1} \price[\good]^t} \right) \left( \frac{\sum_{k \in \goods} \hicksian[\buyer][k]^{t+1} \pricediff[k]}{\sum_{k \in \goods} \hicksian[\buyer][k]^{t+1} \price[k]^t} \right) - \frac{\sum_{\good \in \goods} \hicksian[\buyer][\good]^{t+1} \pricediff[\good]}{\sum_{\good \in \goods} \hicksian[\buyer][\good]^{t+1} \price[\good]^t} \right)
\end{align*}

\noindent
We now use the bound $x \geq \log \left( 1 + x \right)$, with $x = \frac{4}{3} \left(\frac{\sum_{\good \in \goods} \hicksian[\buyer][\good]^{t+1} \pricediff[\good]}{\sum_{\good \in \goods} \hicksian[\buyer][\good]^{t+1} \price[\good]^t} \right) \left(\frac{\sum_{k \in \goods} \hicksian[\buyer][k]^{t+1} \pricediff[k]}{\sum_{k \in \goods} \hicksian[\buyer][k]^{t+1} \price[k]^t} \right) - \frac{\sum_{\good \in \goods} \hicksian[\buyer][\good]^{t+1} \pricediff[\good]}{\sum_{\good \in \goods} \hicksian[\buyer][\good]^{t+1} \price[\good]^t}$ to get:
\begin{align*}
    & \budget[\buyer] \log \left(1  + \frac{4}{3} \left( \frac{\sum_{\good \in \goods} \hicksian[\buyer][\good]^{t+1} \pricediff[\good]}{\sum_{\good \in \goods} \hicksian[\buyer][\good]^{t+1} \price[\good]^t} \right) \left(\frac{\sum_{k \in \goods} \hicksian[\buyer][k]^{t+1} \pricediff[k]}{\sum_{k \in \goods} \hicksian[\buyer][k]^{t+1} \price[k]^t} \right) - \frac{\sum_{\good \in \goods} \hicksian[\buyer][\good]^{t+1} \pricediff[\good]}{\sum_{\good \in \goods} \hicksian[\buyer][\good]^{t+1} \price[\good]^t}\right)\\
    &\leq \budget[\buyer] \left( \frac{4}{3} \left( \frac{\sum_{\good \in \goods} \hicksian[\buyer][\good]^{t+1} \pricediff[\good]}{\sum_{\good \in \goods} \hicksian[\buyer][\good]^{t+1} \price[\good]^t} \right) \left( \frac{\sum_{k \in \goods} \hicksian[\buyer][k]^{t+1} \pricediff[k]}{\sum_{k \in \goods} \hicksian[\buyer][k]^{t+1} \price[k]^t} \right) - \frac{\sum_{\good \in \goods} \hicksian[\buyer][\good]^{t+1} \pricediff[\good]}{\sum_{\good \in \goods} \hicksian[\buyer][\good]^{t+1} \price[\good]^t} \right)\\
    &= \frac{4}{3} \budget[\buyer] \left( \frac{\sum_{\good \in \goods} \hicksian[\buyer][\good]^{t+1} \pricediff[\good]}{\sum_{\good \in \goods} \hicksian[\buyer][\good]^{t+1} \price[\good]^t} \right) \left( \frac{\sum_{k \in \goods} \hicksian[\buyer][k]^{t+1} \pricediff[k]}{\sum_{k \in \goods} \hicksian[\buyer][k]^{t + 1} \price[k]^t} \right) - \budget[\buyer] \left( \frac{\sum_{\good \in \goods} \hicksian[\buyer][\good]^{t+1} \pricediff[\good]}{\sum_{\good \in \goods} \hicksian[\buyer][\good]^{t+1} \price[\good]^t} \right) \\
    &\leq \frac{4}{3} \budget[\buyer] \left( \frac{\sum_{\good \in \goods} \hicksian[\buyer][\good]^{t+1} \pricediff[\good]}{\sum_{\good \in \goods} \hicksian[\buyer][\good]^{t} \price[\good]^t} \right) \left( \frac{\sum_{k \in \goods} \hicksian[\buyer][k]^{t+1} \pricediff[k]}{\sum_{k \in \goods} \hicksian[\buyer][k]^{t} \price[k]^t} \right) - \budget[\buyer] \left( \frac{\sum_{\good \in \goods} \hicksian[\buyer][\good]^{t+1} \pricediff[\good]}{\sum_{\good \in \goods} \hicksian[\buyer][\good]^{t+1} \price[\good]^t} \right) && \text{(\Cref{hicksian-is-expend-minimizer})} \\
    &\leq \frac{4}{3} \budget[\buyer] \left( \frac{\sum_{\good \in \goods} \hicksian[\buyer][\good]^{t} \pricediff[\good]}{\sum_{\good \in \goods} \hicksian[\buyer][\good]^{t} \price[\good]^t} \right) \left( \frac{\sum_{k \in \goods} \hicksian[\buyer][k]^{t} \pricediff[k]}{\sum_{k \in \goods} \hicksian[\buyer][k]^{t} \price[k]^t} \right) - \budget[\buyer] \left( \frac{\sum_{\good \in \goods} \hicksian[\buyer][\good]^{t+1} \pricediff[\good]}{\sum_{\good \in \goods} \hicksian[\buyer][\good]^{t+1} \price[\good]^t} \right) && \text{(\Cref{law-of-demand-corollary})} \\
    &= \frac{4}{3} \frac{1}{\budget[\buyer]} \left( \sum_{\good \in \goods} \pricediff[\good] \frac{ \budget[\buyer] \hicksian[\buyer][\good]^{t} }{\sum_{\good \in \goods} \hicksian[\buyer][\good]^{t} \price[\good]^t} \right) \left( \sum_{k \in \goods} \pricediff[k]  \frac{ \budget[\buyer] \hicksian[\buyer][k]^{t} }{\sum_{k \in \goods} \hicksian[\buyer][k]^{t} \price[k]^t} \right) - \sum_{\good \in \goods} \pricediff[\good] \left( \frac{ \budget[\buyer] \hicksian[\buyer][\good]^{t+1} }{\sum_{\good \in \goods} \hicksian[\buyer][\good]^{t+1} \price[\good]^t} \right) \\
    &= \frac{4}{3} \frac{1}{\budget[\buyer]} \left( \sum_{\good \in \goods} \pricediff[\good]  \demand[\buyer][\good]^t \right) \left( \sum_{k \in \goods} \pricediff[k] \demand[\buyer][k]^t \right) - \sum_{\good \in \goods} \pricediff[\good] \left(\frac{ \budget[\buyer] \hicksian[\buyer][\good]^{t+1} }{\sum_{\good \in \goods} \hicksian[\buyer][\good]^{t+1} \price[\good]^t} \right) && \text{(\Cref{equiv-def-demand})}\\
    &\leq \frac{4}{3} \frac{1}{\budget[\buyer]} \sum_{\good \in \goods}\sum_{k \in \goods}   \demand[\buyer][\good]^t\demand[\buyer][k]^t  |\pricediff[\good]||\pricediff[k]| -\sum_{\good \in \goods} \pricediff[\good] \left( \frac{ \budget[\buyer] \hicksian[\buyer][\good]^{t+1} }{\sum_{\good \in \goods} \hicksian[\buyer][\good]^{t+1} \price[\good]^t} \right) \\
    &\leq \frac{4}{3} \sum_{\good \in \goods} \demand[\buyer][\good]^t \left( \frac{(\pricediff[\good])^2}{\price[\good]^t} \right) - \sum_{\good \in \goods} \pricediff[\good] \left( \frac{ \budget[\buyer] \hicksian[\buyer][\good]^{t+1} }{\sum_{\good \in \goods} \hicksian[\buyer][\good]^{t+1} \price[\good]^t}\right) && \text{(\Cref{leontief-ineq})}
\end{align*}
\end{proof}

\ineqdevanur*
\begin{proof}[\Cref{ineq-devanur}]
\begin{align*}
&\potential(\price^{t+1}) - \lapprox[\potential][\price^{t+1}][\price^t]\\
&= \potential(\price^{t+1}) - \potential(\price^t) + \excess(\price^t) \cdot \left(\price^{t+1} - \price^t\right)\\
&= \sum_{\good \in \goods} \left( \price[\good]^t + \pricediff[\good] \right) - \sum_{\buyer \in \buyers} \budget[\buyer] \log \left( \expend[\buyer](\price^t + \pricediff, 1)\right) - \sum_{\good \in \goods} \price[\good]^t + \sum_{\buyer \in \buyers} \budget[\buyer] \log \left( \expend[\buyer](\price^t , 1)\right) + \sum_{\good \in \goods} \excess[\good](\price^t) \pricediff[\good]\\
&= \sum_{\good \in \goods} \left( \price[\good]^t + \pricediff[\good] \right) - \sum_{\buyer \in \buyers} \budget[\buyer] \log \left( \expend[\buyer](\price^t + \pricediff, 1)\right) - \sum_{\good \in \goods} \price[\good]^t + \sum_{\buyer \in \buyers} \budget[\buyer] \log \left( \expend[\buyer](\price^t , 1)\right) + \sum_{\good \in \goods} (\demand[\good]^t - 1) \pricediff[\good]\\
&=  \sum_{\good \in \goods} \pricediff[\good] \demand[\good]^t - \sum_{\buyer \in \buyers} \budget[\buyer] \log \left( \expend[\buyer](\price^t + \pricediff, 1)\right) + \sum_{\buyer \in \buyers} \budget[\buyer] \log \left( \expend[\buyer](\price^t , 1)\right) \\
&= \sum_{\good \in \goods} \pricediff[\good] \demand[\good]^t + \sum_{\buyer \in \buyers} \budget[\buyer] \log \left( \frac{\expend[\buyer](\price^t, 1)}{\expend[\buyer](\price^t + \pricediff, 1)}\right)
\end{align*}

Recall that the expenditure at any price $\price$ is equal to the sum of the product of the Hicksian demands and the prices; that is, $\expend[\buyer](\price^t, 1) = \sum_{\good \in \goods} \hicksian[\buyer][\good]^t \price[\good]^t$. We then have:
\begin{align*}
    &\sum_{\good \in \goods} \pricediff[\good] \demand[\good]^t + \sum_{\buyer \in \buyers} \budget[\buyer] \log \left( \frac{\expend[\buyer](\price^t, 1)}{\expend[\buyer](\price^t + \pricediff, 1)}\right)\\
    &= \sum_{\good \in \goods} \pricediff[\good] \demand[\good]^t + \sum_{\buyer \in \buyers} \budget[\buyer] \log \left( \frac{\sum_{\good \in \goods} \hicksian[\buyer][\good]^{t} \price[\good]^t}{\sum_{\good \in \goods} \hicksian[\buyer][\good]^{t+1} \left( \price[\good]^t + \pricediff[\good]\right)}\right)\\
    &= \sum_{\good \in \goods} \pricediff[\good] \demand[\good]^t + \sum_{\buyer \in \buyers} \budget[\buyer] \log \left( \frac{\sum_{\good \in \goods} \hicksian[\buyer][\good]^{t} \price[\good]^t}{\sum_{\good \in \goods} \hicksian[\buyer][\good]^{t+1}  \price[\good]^t + \sum_{\good \in \goods} \hicksian[\buyer][\good]^{t+1} \pricediff[\good]}\right)\\
    &\leq \sum_{\good \in \goods} \pricediff[\good] \demand[\good]^{t} + \sum_{\buyer \in \buyers} \budget[\buyer] \log \left( \frac{\sum_{\good \in \goods} \hicksian[\buyer][\good]^{t+1} \price[\good]^{t}}{\sum_{\good \in \goods} \hicksian[\buyer][\good]^{t+1}  \price[\good]^t + \sum_{\good \in \goods} \hicksian[\buyer][\good]^{t+1} \pricediff[\good]}\right) && \text{(\Cref{hicksian-is-expend-minimizer})}\\
    &= \sum_{\good \in \goods} \pricediff[\good] \demand[\good]^{t} + \sum_{\buyer \in \buyers} \budget[\buyer] \log \left( 1 - \frac{\sum_{\good \in \goods} \hicksian[\buyer][\good]^{t+1} \pricediff[\good]}{\sum_{\good \in \goods} \hicksian[\buyer][\good]^{t+1} \price[\good]^t} \left( 1 + \frac{\sum_{\good \in \goods} \hicksian[\buyer][\good]^{t+1} \pricediff[\good]}{\sum_{\good \in \goods} \hicksian[\buyer][\good]^{t+1} \price[\good]}\right)^{-1} \right),
\end{align*}

\noindent
where the last line is obtained by simply noting that $\forall a, b \in \R, \frac{a}{a+b} = 1 - \frac{b}{a}(1+ \frac{b}{a})^{-1}$. 
Continuing,
\begin{align}
    &\sum_{\good \in \goods} \pricediff[\good] \demand[\good]^{t} + \sum_{\buyer \in \buyers} \budget[\buyer] \log \left( 1 - \frac{\sum_{\good \in \goods} \hicksian[\buyer][\good]^{t+1} \pricediff[\good]}{\sum_{\good \in \goods} \hicksian[\buyer][\good]^{t+1} \price[\good]^t} \left( 1 + \frac{\sum_{\good \in \goods} \hicksian[\buyer][\good]^{t+1} \pricediff[\good]}{\sum_{\good \in \goods} \hicksian[\buyer][\good]^{t+1} \price[\good]}\right)^{-1}  \right)\\ 
    &\leq \sum_{\good \in \goods} \pricediff[\good] \demand[\good]^{t} + \sum_{\buyer \in \buyers} \left[ \frac{4}{3} \sum_{\good \in \goods} \demand[\buyer][\good]^t \left( \frac{(\pricediff[\good])^2}{\price[\good]^t} \right) - \sum_{\good \in \goods} \pricediff[\good] \left( \frac{\budget[\buyer] \hicksian[\buyer][\good]^{t+1}}{\sum_{\good \in \goods} \hicksian[\buyer][\good]^{t+1} \price[\good]^t} \right) \right] && \text{(\Cref{fix-buyer-bound})}\\
    &= \sum_{\good \in \goods} \sum_{\buyer \in \buyers} \pricediff[\good] \demand[\buyer][\good]^{t} - \sum_{\buyer \in \buyers} \sum_{\good \in \goods} \pricediff[\good] \left( \frac{ \budget[\buyer] \hicksian[\buyer][\good]^{t+1} }{\sum_{\good \in \goods} \hicksian[\buyer][\good]^{t+1} \price[\good]^t} \right) + \frac{4}{3} \sum_{\buyer \in \buyers}  \sum_{\good \in \goods} \demand[\buyer][\good]^t \left( \frac{(\pricediff[\good])^2}{\price[\good]^t} \right) \\
    &= \sum_{\good \in \goods} \sum_{\buyer \in \buyers}  \pricediff[\good] \left( \frac{ \budget[\buyer] \hicksian[\buyer][\good]^{t} }{\sum_{\good \in \goods} \hicksian[\buyer][\good]^{t} \price[\good]^t} \right) - \sum_{\buyer \in \buyers} \sum_{\good \in \goods} \pricediff[\good] \left( \frac{ \budget[\buyer] \hicksian[\buyer][\good]^{t+1} }{\sum_{\good \in \goods} \hicksian[\buyer][\good]^{t+1} \price[\good]^t} \right) + \frac{4}{3} \sum_{\buyer \in \buyers}  \sum_{\good \in \goods} \demand[\buyer][\good]^t \left( \frac{(\pricediff[\good])^2}{\price[\good]^t} \right) && \text{(\Cref{equiv-def-demand})} \\
    &= \sum_{\buyer \in \buyers}  \sum_{\good \in \goods} \left[ \frac{\budget[\buyer] \pricediff[\good] \hicksian[\buyer][\good]^{t}}{\sum_{l \in \goods} \hicksian[\buyer][l]^{t} \price[\good]^t} - \frac{ \budget[\buyer] \pricediff[\good]   \hicksian[\buyer][\good]^{t+1}}{\sum_{r \in \goods} \hicksian[\buyer][r]^{t+1} \price[r]^t} \right] + \frac{4}{3} \sum_{\buyer \in \buyers}  \sum_{\good \in \goods} \demand[\buyer][\good]^t \left( \frac{(\pricediff[\good])^2}{\price[\good]^t} \right) \\
    &= \sum_{\buyer \in \buyers} \sum_{\good \in \goods} \left[ \frac{\budget[\buyer] \pricediff[\good] \hicksian[\buyer][\good]^{t} \left( \sum_{k \in \goods} \hicksian[\buyer][k]^{t+1} \price[k]^t \right) - \budget[\buyer]\pricediff[\good] \hicksian[\buyer][\good]^{t+1} \left(\sum_{k \in \goods} \hicksian[\buyer][k]^{t} \price[k]^t \right)}{\left( \sum_{l \in \goods} \hicksian[\buyer][l]^{t} \price[l]^t \right) \left( \sum_{r \in \goods} \hicksian[\buyer][r]^{t+1} \price[r]^t \right) } \right] + \frac{4}{3} \sum_{\buyer \in \buyers} \sum_{\good \in \goods} \demand[\buyer][\good]^t \left( \frac{(\pricediff[\good])^2}{\price[\good]^t} \right) \\
    &= \frac{\sum_{\buyer,\good, k} \left( \budget[\buyer] \pricediff[\good]  \hicksian[\buyer][k]^{t+1} \hicksian[\buyer][\good]^{t} \price[k]^t \right)  -  \sum_{\buyer,\good, k} \left( \budget[\buyer] \pricediff[\good] \hicksian[\buyer][\good]^{t+1} \hicksian[\buyer][k]^{t} \price[k]^t \right) }{\left( \sum_{l \in \goods} \hicksian[\buyer][l]^{t} \price[l]^t \right) \left(\sum_{r \in \goods} \hicksian[\buyer][r]^{t+1} \price[r]^t \right)} +  \frac{4}{3} \sum_{\buyer \in \buyers}   \sum_{\good \in \goods} \demand[\buyer][\good]^t \left( \frac{(\pricediff[\good])^2}{\price[\good]^t} \right) \\
    &= 0 + \frac{4}{3} \sum_{\buyer \in \buyers}   \sum_{\good \in \goods} \demand[\buyer][\good]^t \left( \frac{(\pricediff[\good])^2}{\price[\good]^t} \right) \\
    &= \frac{4}{3} \sum_{\good \in \goods} \left[ \demand[\good]^{t} \left( \frac{(\pricediff[\good])^2}{\price[\good]^t} \right) \right] \\
    &= \frac{4}{3} \sum_{\good \in \goods}  \demand[\good]^{t} \left( \frac{9}{2} \right) \divergence[\mathrm{KL}][{\price[\good]^t + \pricediff[\good]}][{\price[\good]^t}]  && \text{(\Cref{kl-divergence-1})} \\
    &= 6 \sum_{\good \in \goods}  \demand[\good]^{t} \divergence[\mathrm{KL}][{\price[\good]^t + \pricediff[\good]}][{\price[\good]^t}]  \\
    &\leq 6 \max_{\substack{\good \in \goods\\ t \in \N}} \{\demand[\good]^{t}\}\sum_{\good \in \goods}   \divergence[\mathrm{KL}][{\price[\good]^t + \pricediff[\good]}][{\price[\good]^t}]  \\
    &= 6 \max_{\substack{\good \in \goods\\ t \in \N}} \{\demand[\good]^{t}\} \ \divergence[\mathrm{KL}][{\price^t + \pricediff}][{\price^t}] 
\end{align}
\end{proof}

% \restoregeometry
% Removed proposition which was included for intuition
% \begin{proposition}
% There exists a constant $c >0$, such that throughout the tatonnement algorithm we have that $\forall t \in \N, \ \ \demand[\good]^t \leq c$.
% \end{proposition}

% \begin{proof}
% The demand for a good $\good$ can be unbounded iff the budget of a buyer is infinite or the price $\price[\good]$ of good $\good$, $\price[\good] = 0$. This can be directly seen from the definition of the Marshallian demand. By the assumption of the model, we know that no buyer has an infinite budget. Hence, the only way for a good to have an unbounded demand is for the tatonnement process to assign a price of $0$ for good $\good$. This, however, is impossible. This is because when the good is supplied in excess the algorithm reduced the price of good $\good$ until the good is no more supplied in excess. Since reducing the price of a good always increases its demand or keeps it constant, after a certain amount of price updates, the supply of the good $\good$ is guaranteed to no more be in excess. Hence, in order for the price of a good to be $0$ throughout the algorithm, we would need the price update to "overshoot" and set the price to $0$, However, $e^{\frac{\excess(\price(t))}{\gamma}} = 0$ cannot happen in one update since $e^{\frac{\excess(\price(t))}{\gamma}} \to \infty$ only when $\frac{\excess(\price(t))}{\gamma} \to - \infty$ which is impossible in one iteration of the algorithm. Hence, the demand throughout the algorithm must be bounded by some constant.
% \end{proof}

\begin{lemma}
\label{gc-max-increase-one-round}
Suppose that 
% $\frac{|\pricediff[\good]|}{\price[\good]^t} \leq \frac{1}{4}$ and
the entropic t\^atonnement process 
% given in \Cref{tatonnement-KL} and \Cref{tatonnement-KL2} 
is run on a gross complements CCH Fisher markets with $\gamma = 5 \max_{t \in \N, \good \in \goods} \{\demand[\good]^t\}$, then the change in the demand for any good $\good$ in one iteration is bounded such that:
\begin{align}
    &\forall  \good \in \goods &e^{\frac{1}{5}} \demand[\good]^t \geq \demand[\good]^{t+1} \geq e^{- \frac{1}{5}} \demand[\good]^t
\end{align}
\end{lemma}
\begin{proof}[\Cref{gc-max-increase-one-round}]
Since in gross complements markets the demand for a good $\good$ increases when the price $\price[k]$ of other goods $k \neq \good$ decrease, the most that the demand of good $\good$ can increase in one iteration is when the prices of all goods decrease. By \Cref{price-change}, our t\^atonnement update rule ensures that in one iteration prices do not change more than $e^{-\frac{1}{5}} \price[\good]^{t}\leq \price[\good]^{t+1} \leq e^{\frac{1}{5}} \price[\good]^{t} $. Thus, we can bound the increase in the demand of a good $\good$ due to changes in the prices of all other goods in one round as follows:
\begin{align*}
    \demand[\good]^{t+1} &= \sum_{\buyer \in  \buyers} \marshallian[\buyer][\good](\price^{t+1}, \budget[\buyer])\\
    &\leq \sum_{\buyer \in  \buyers} \marshallian[\buyer][\good](e^{-\frac{1}{5}}\price^{t}, \budget[\buyer])\\
    &= \sum_{\buyer \in  \buyers} \argmax_{\allocation[\buyer]: \allocation[\buyer] \cdot e^{-\frac{1}{5}} \price^t \leq \budget[\buyer]} \util[\buyer](\allocation[\buyer])\\
    &= \sum_{\buyer \in  \buyers} \argmax_{\allocation[\buyer]: \allocation[\buyer] \cdot \price^t \leq e^{\frac{1}{5}}\budget[\buyer]} \util[\buyer](\allocation[\buyer])\\
    &=  \sum_{\buyer \in  \buyers} \marshallian[\buyer][\good](\price^{t}, e^{\frac{1}{5}}\budget[\buyer])\\
    &= e^{\frac{1}{5}} \sum_{\buyer \in  \buyers} \marshallian[\buyer][\good](\price^{t}, \budget[\buyer]) && \text{(\Cref{homo-indirect-util})}\\
    &= e^{\frac{1}{5}} \demand[\good]^t 
\end{align*}

% \enr{
% \begin{itemize}
%     \item[(\ref{lemmaB-1})] Definition of demand. 
%     \item[(\ref{lemmaB-2})] As you decrease prices, demand increases.
%     \item[(\ref{lemmaB-3})] definition of demand. 
%     \item[(\ref{lemmaB-4})] some manipulation over the domand of the argmax
%     \item[(\ref{lemmaB-5})] back to the demand
%     \item[(\ref{lemmaB-6})] definition
% \end{itemize}

% Ok, this proof can be significantly shortened. I think you already had some facts for manipulating the domain of the argmax WAY WAY before :) Can't you use them here? I feel like there is a point where such long proofs impede understanding what is going on :(. But don't get me wrong, definitely spelling things out is great. At the same time, knowing the exact level of details to write is kind of an art, isn't it?
% }

Similarly, the demand for $\good$ decreases the most when the prices of all goods go up by a factor of $e^{\frac{1}{5}}$, hence the maximum decrease of the demand for good $\good$ in one iteration is by a factor of $e^{-\frac{1}{5}}$.
\end{proof}

Using the result obtained in \Cref{gc-max-increase-one-round}, we bound the demand for any good throughout the t\^atonnement algorithm. We also include a comparison of our bound to \citeauthor{fisher-tatonnement}'s bound for Leontief markets.

\begin{lemma}\label{demand-ub-gc}
For all gross complements CCH Fisher markets, if the entropic t\^atonnement process 
% with KL-Divergence given in \Cref{tatonnement-KL} and \Cref{tatonnement-KL2} 
is run such that for all goods $\frac{|\pricediff[\good]|}{\price[\good]^t} \leq \frac{1}{4}$ holds, then the demand for any good $\good \in \goods$ during the algorithm is bounded such that:
\begin{align*}
    \max_{t \in N}\left\{ \demand[\good]^t \right\}\leq \max_{k \in \goods} \frac{\demand[\good]^0}{  \demand[k]^0} \enspace .
\end{align*} 
% \enr{as usual, I worry about division by 0 a lot :) -- (I was once trained as a math teacher, I guess that is why jaajjaj!). Are we sure that the denominator of this bound is always non-zero? if so, just delete my comment and add a line about it after the lemma. Something like, note that this bound is meaningful as the denominator is never zero. Now, how small can it be?? if it is super duper small, the bound is less and less meaningful. I think this is another opportunity for numerical experimentation. }
\end{lemma}

\begin{proof}[\Cref{demand-ub-gc}]
By the definition of the t\^atonnement process if the demand of a good is under 1, its price must decrease and if the demand of a good is over 1, its price must increase. Since we are dealing with gross complement markets, a decrease in the price of any good leads to an increase in the demand for good $\good$. This also means that if the demand of all goods is over 1, then the demand of all goods must decrease in the next iteration. We proceed with proof by cases.

\underline{Case 1: There exists a good whose initial demand is under 1, i.e., $\exists k \in \goods$ s.t. $\demand[k]^0 < 1$}\\
We want to find the highest demand for good $\good$ when there exists a good whose initial demand is less than 1.
From \Cref{gc-max-increase-one-round}, we know that the demand of good $\good$ increases the most in one round when the prices of all goods decreases by a factor of $e^{-\frac{1}{5}}$. We can then upper bound the maximum demand for good $\good$ when there exists a good whose demand is under 1 by decreasing the prices of all goods by a factor of $e^{-\frac{1}{5}}$ repeatedly until the demand for all goods exceeds 1. 
% Once the demands of all goods are above 1, in the next round we are guaranteed that prices of all goods will go up, i.e., their demands will go down, and since we had increased the demands of all by the maximum factor of $e^{\frac{1}{5}}$ we know that the demand of goods cannot go any higher. 
Let $k \in \N$ be the number of iteration necessary until the demand of all goods exceeds 1, we want to find $k \in \N$ such that $(e^{\frac{1}{5}})^k \min_{\good \in \goods} \demand[\good]^0 \geq 1$. That is, we want to figure out how many iterations it will take until the demand of the good with the minimum initial demand exceeds 1:
\begin{align*}
    e^{(\frac{1}{5})^k}  \min_{\good \in \goods} \demand[\good]^0 &\geq 1 \\
    e^{\frac{k}{5}}  \min_{\good \in \goods} \demand[\good]^0 &\geq 1\\
    e^{\frac{k}{5}}   &\geq \frac{1}{\min_{\good \in \goods} \demand[\good]^0}\\
    \frac{k}{5} &\geq \log\left( \frac{1}{\min_{\good \in \goods} \demand[\good]^0} \right)\\
    k &\geq  - 5\log\left( \min_{\good \in \goods} \demand[\good]^0 \right)
\end{align*}
\noindent
where $\min_{\good \in \goods} \demand[\good]^0 > 0$ since for gross complements markets the demand for any good can only be 0 if the price is infinite which is impossible by our update rule. Note that since we are dealing with discrete update steps the number of iterations that can maximally increase the demand of good $\good$ is $\lceil - 5\log\left( \min_{\good \in \goods} \demand[\good]^0 \right) \rceil$. We can overestimate this quantity by simply noting $\lceil - 5\log\left( \min_{\good \in \goods} \demand[\good]^0 \right) \rceil \leq - 5\log\left( \min_{\good \in \goods} \demand[\good]^0 \right) + 1$.

Hence, combining these number of iteration with the increase factor, we can obtain the the highest value the demand of good $\good$ can reach throughout t\^atonnement:
\begin{align*}
    e^{(\frac{1}{5})^k}\demand[\good]^0 &=e^{(\frac{1}{5})^{- 5\log\left( \min_{k \in \goods} \demand[k]^0 \right) + 1}}\demand[\good]^0 \\
    % &=e^{\frac{- 5\log\left( \min_{k \in \goods} \demand[k]^0 \right) + 1}{5}}\demand[\good]^0\\
    % &=e^{- \log\left( \min_{k \in \goods} \demand[\good]^0 \right) + \frac{1}{5}}\demand[\good]^0\\
    % &=e^{\frac{1}{5}} e^{- \log\left( \min_{k \in \goods} \demand[\good]^0 \right)} \demand[\good]^0\\
    % &=e^{\frac{1}{5}} \frac{1}{ \min_{k \in \goods} \demand[k]^0}\demand[\good]^0\\
    &= e^{\frac{1}{5}}\frac{\demand[\good]^0}{ \min_{k \in \goods} \demand[k]^0}\\
    &= e^{\frac{1}{5}} \max_{k \in \goods} \frac{\demand[\good]^0}{  \demand[k]^0}\\
    &\leq 2 \max_{k \in \goods} \frac{\demand[\good]^0}{  \demand[k]^0}
\end{align*}
\noindent
where $\min_{\good \in \goods} \demand[\good]^0 > 0$ once again.

The above demand for good $\good$ is maximal because it takes into account the worst amount by which the demand for good $\good$ can increase in each iteration, which combined with the associated maximum number of iterations gives the upper bound on the demand of good $\good$ throughout the algorithm.

\underline{Case 2: All goods have initial demand greater than or equal to 1, i.e., $\forall \good \in \goods, \ \ \demand[\good]^0 \geq 1$}

% It is possible at the initialization of the t\^atonnement process that the demand of all other\enr{which others?? the assumption here is that all goods have demand at least 1} goods is above 1, in which case the prices of other goods can only increase and hence the demand of good $\good$ can only decrease in the next iteration. Our experiments\enr{without including the experiments, this sentence is meaningless} suggest that the demand for good $\good$ will keep going down in the following iterations as well making $\demand[\good]^0$ the upper bound. However we are not able to provide a proof of this conjecture \senr{and}{and,} as a result \enr{result,} settle for the following loser bound proof \enr{I think we can settle for a loser bound but not for a loser bound proof}:

From \Cref{gc-max-increase-one-round}, we know that the most that the demand of any good $k \in \goods$ can decrease is by a factor of $e^{-\frac{1}{5}}$. Hence, in the worst case the demand of any good can decrease to at most $e^{-\frac{1}{5}}$. In that case, in the round following the decrease in the demand, the demand of good $\good$ can at most increase to $e^{\frac{1}{5}}\demand[\good]^0$. Such an update would, however, also require the demand of other goods to go over 1 since $e^{-\frac{1}{5}} e^{\frac{1}{5}} = 1$. This means that there can only be one iteration of such a maximal update. As a result, when the demand of all goods is over 1, the demand throughout the algorithm is bounded by:
\begin{align*}
    \demand[\good]^t \leq e^{\frac{1}{5}} \demand[\good]^0 \leq 2\demand[\good]^0
\end{align*}

This gives us an overall bound for the highest the demand of any good $\good$ can reach:
\begin{align*}
    \demand[\good]^t &\leq \max\left\{ 2\demand[\good]^0, 2 \max_{k \in \goods} \frac{\demand[\good]^0}{  \demand[k]^0} \right\}\\
    &\leq 2 \max\left\{ \demand[\good]^0, \max_{k \in \goods} \frac{\demand[\good]^0}{\demand[k]^0} \right\}\\
    &\leq 2  \max_{k \in \goods} \frac{\demand[\good]^0}{\demand[k]^0} 
\end{align*}
\noindent
where $\min_{\good \in \goods} \demand[\good]^0 > 0$.

\emph{Comparison to Leontief Demand Upper Bound}\\
For Leontief markets, \citeauthor{fisher-tatonnement} gave a $\max_{k} \frac{\valuation[\buyer][\good]}{\valuation[\buyer][k]}$ upper bound, for arbitrary $\buyer \in \buyers$ ,on the value of the demand of $\good$ throughout t\^atonnement which holds for for any buyer $\buyer$ \cite{fisher-tatonnement}. Since our bound is a generalization of their result for a larger class of markets including Leontief markets, we present a comparison by showing what our bound implies for Leontief markets.
% Our bound must be most likely higher than their bound for Leontief markets since we have less information then them on the market (although it is possible that their bound might not be tight) and ideally not too large so as to not add an extra constant to the convergence of the t\^atonnement process.
% Let's check how our bound performs. 
For the Leontief case, our upper bound gives us:
\begin{align*}
    2\max_{k \in \goods} \frac{\demand[\good]^0}{  \demand[k]^0} &= 2\max_{k \in \goods} \frac{\sum_{\buyer \in \buyers}\frac{\budget[\buyer] \valuation[\buyer][\good]}{\sum_{\good \in \goods} \price[\good]^0 \valuation[\buyer][\good]}}{\sum_{\buyer \in \buyers}\frac{\budget[\buyer] \valuation[\buyer][k]}{\sum_{\good \in \goods} \price[\good]^0 \valuation[\buyer][\good]}} \geq 2\max_{k \in \goods} \min_{\buyer \in \buyers} \frac{\frac{\budget[\buyer] \valuation[\buyer][\good]}{\sum_{\good \in \goods} \price[\good]^0 \valuation[\buyer][\good]}}{\frac{\budget[\buyer] \valuation[\buyer][k]}{\sum_{\good \in \goods} \price[\good]^0 \valuation[\buyer][\good]}} \geq 2 \max_{k \in \goods} \min_{\buyer \in \buyers} \frac{ \valuation[\buyer][\good]}{\valuation[\buyer][k]} 
\end{align*}

Similarly, we can also obtain $ 2 \max_{k \in \goods} \max_{\buyer \in \buyers} \frac{ \valuation[\buyer][\good]}{\valuation[\buyer][k]} \geq 2 \max_{k \in \goods} \frac{\demand[\good]^0}{  \demand[k]^0} $. This means that the upper bound on the demand we obtained for the Leontief market reduces to the upper bound provided by \citeauthor{fisher-tatonnement}.
% \enr{I think this subsection 'Compariosn to Leontief Demand Upper Bound, should be short and to the point, i.e., our bound reduces to Cheung et al bounds. A couple of lines maximum}
\end{proof}

We now proceed to upper bound the demand of any good throughout t\^atonnement in gross substitutes markets. To do so, we first lower bound the maximum change in the demand of a good in one round.

\begin{lemma}\label{gs-max-increase-one-round}
Suppose that 
% $\frac{|\pricediff[\good]|}{\price[\good]^t} \leq \frac{1}{4}$ and
the entropic t\^atonnement process 
% given in \Cref{tatonnement-KL} and \Cref{tatonnement-KL2} 
is run on a gross substitutes Fisher market with $$\gamma = 5 \max\limits_{\substack{t \in \N \\ \good \in \goods}} \{\demand[\good]^t\} \enspace ,$$ then the \textbf{maximum increase} in the demand for any good $\good$ in one iteration is bounded such that:
\begin{align*}
    \demand[\good]^{t+1} \geq e^{\frac{1}{5}} \demand[\good]^{t} enspace ,
\end{align*}
and the \textbf{maximum decrease} in the demand in one iteration is bounded such that: 
\begin{align*}
    \demand[\good]^{t+1} \leq e^{-\frac{1}{5}} \demand[\good]^{t} \enspace .
\end{align*}
\end{lemma}

\begin{proof}[\Cref{gs-max-increase-one-round}]
The maximum change in the demand of good $\good$ in one iteration due to a decrease in the price of good $\good$, can be lower bounded by decreasing all the prices by a factor of $e^{-\frac{1}{5}}$, i.e., the most the prices can decrease by in one iteration, since decreasing the prices of other goods decreases the demand of good $\good$. That is, we have:
\begin{align*}
    \demand[\good]^{t+1} &= \sum_{\buyer \in  \buyers} \marshallian[\buyer][\good](\price^{t+1}, \budget[\buyer])\\
    &\geq \sum_{\buyer \in  \buyers} \marshallian[\buyer][\good](e^{-\frac{1}{5}}\price^{t}, \budget[\buyer])\\
    &= \sum_{\buyer \in  \buyers} \argmax_{\allocation[\buyer]: \allocation[\buyer] \cdot e^{-\frac{1}{5}} \price^t \leq \budget[\buyer]} \util[\buyer](\allocation[\buyer])\\
    &= \sum_{\buyer \in  \buyers} \argmax_{\allocation[\buyer]: \allocation[\buyer] \cdot \price^t \leq e^{\frac{1}{5}}\budget[\buyer]} \util[\buyer](\allocation[\buyer])\\
    &=  \sum_{\buyer \in  \buyers} \marshallian[\buyer][\good](\price^{t}, e^{\frac{1}{5}}\budget[\buyer])\\
    &= e^{\frac{1}{5}} \sum_{\buyer \in  \buyers} \marshallian[\buyer][\good](\price^{t}, \budget[\buyer]) && \text{(\Cref{homo-expend})}\\
    &= e^{\frac{1}{5}} \demand[\good]^t
\end{align*}

That is, the maximum demand that good $\good$ can reach due to a maximum decrease only in its price in one iteration is lower bounded by $e^{\frac{1}{5}}$. This is a lower bound because all prices went down rather than the price of good $\good$ going down and the price all other goods going up. The upper bound for the maximum decrease factor of $e^{- \frac{1}{5}}$ can be shown similarly.
\end{proof}

\begin{lemma}\label{demand-ub-gs}
For all gross substitutes CCH markets, if the entropic t\^atonnement process 
% with KL-Divergence given in \Cref{tatonnement-KL} and \Cref{tatonnement-KL2}
is run such that for all goods $\frac{|\pricediff[\good]|}{\price[\good]^t} \leq \frac{1}{4}$ holds, then the demand for any good $\good \in \goods$ during the algorithm is bounded such that
\begin{align*}
\max_{t \in \N} \left\{\demand[\good]^t \right\} \leq 2 \frac{\sum_{\buyer \in \buyers} \budget[\buyer]}{\price[\good]^0} \max \left\{\max_{k \in \goods}\demand[k]^0,  \frac{\max_{l \in \goods}\demand[l]^0}{\demand[\good]^0} \right\} \enspace .     
\end{align*}

\end{lemma}

\begin{proof}[\Cref{demand-ub-gs}]
We want to find the highest demand for good $\good$ throughout the algorithm. By the definition of the t\^atonnement process if the demand for a good is under 1, its price must decrease and if the price of a good is over 1, it price must increase. Since we are dealing with gross substitutes markets, an increase in the price of goods other than good $\good$ leads to an increase in the demand for good $\good$, and a decrease in the prices of goods other than good $\good$ leads to a decrease in the demand of good $\good$. 

Before moving further with the proof, note that the demand on any time step $t$ can be upper bounded by dividing the sum of the budgets by the new price of good $\good$ on that time period. This is a simple consequence of Walras' law. That is, the upper bound is simply the case when the consumers decide to spend all their money on good $\good$ instead of the other goods, in which case we know that the consumers cannot spend more than their budget, giving us:
\begin{align}
    \demand[\good]^t \leq \frac{\sum_{\buyer \in \buyers} \budget[\buyer]}{\price[\good]^t}\label{upper-demand-subs}
\end{align}

We now proceed with proof by cases.

\underline{Case 1: The initial demand for good $\good$ is under 1, i.e., $\demand[\good]^0 < 1$.}

Our goal is to understand how high the demand of good $\good$ can reach. To achieve this we will isolate the changes in the demand of good $\good$ caused by the change in the price of goods $\goods \ni k \neq \good$ from the changes in the demand of good $\good$ caused by the changes in the price of good $\good$. The proof proceeds as follows, 1) we use the lower bound for the maximum increase in the demand of good $\good$ caused by a decrease in the price of good $\good$ in one iteration given in \Cref{gs-max-increase-one-round} to upper bound the number of iterations until such maximal decreases in the price of good $\good$ leads the demand of good $\good$ to exceed 1, 2) we use the upper bound on the maximum decrease in the demand of other goods in one iteration caused by increases in the prices of other goods from \Cref{gs-max-increase-one-round}, to upper bound the number of iterations until the demand of all other goods decreases under 1, finally 5) we combine the number of iterations obtained in steps 1 and 2 to lower bound the minimum price of good $\good$ throughout the algorithm, which we then combine with \Cref{upper-demand-subs} to obtain an  upper bound on the demand of good $\good$ throughout the t\^atonnement algorithm. 

First, we would like to upper bound the number of iterations during which the demand of good $\good$ increases maximally until it exceeds a demand of 1. Since from \Cref{gs-max-increase-one-round}, we have a lower bound on the maximum increase in the demand of good $\good$ caused by a decrease in the price of good $\good$, we can calculate an upper bound on the number of such maximum demand increasing iterations until the demand of good $\good$ exceeds 1. Let $k$ be the upper bound on the number of iterations needed until the demand of good $k$ is greater than or equal to 1, we have:
\begin{align}
    {e^{\frac{1}{5}}}^k \demand[\good]^0 \geq 1 \nonumber \\
    e^{\frac{k}{5}}\demand[\good]^0 \geq 1 \nonumber \\
    e^{\frac{k}{5}} \geq \frac{1}{\demand[\good]^0} \nonumber \\
    \frac{k}{5} \geq -\log\left(\demand[\good]^0\right)\nonumber \\
    k \geq -5\log\left(\demand[\good]^0\right)\label{max-num-iter-1}
\end{align}

That is the number of maximum demand increasing iterations for good $\good$ is upper bounded by $5\log\left(\demand[\good]^0\right)$. 

\emph{So far}, we have calculated how many maximally price decreasing iterations we need for the demand of good $\good$ to exceed 1. However, it is also possible that in some iterations the decreases in the prices of other goods might increase their demand and as a result decrease the demand of good $\good$ so that its demand stays under under 1 and its price keeps decreasing. That is why we also need to find an upper bound on the number of iterations during which the price of $\good$ can still be maximally decreasing until all other goods reach a demand that is under 1. To do so, we use \Cref{gs-max-increase-one-round}'s upper bound on the decrease in the demand of other goods when their prices are increased to calculate an upper bound on the number of such iterations. 

First, note that the demand obtained by increasing the prices of all goods is a upper bound to the maximum amount by which the demand of any good can maximally decrease in one iteration since we are in a gross substitutes market. That is, when increasing the price of one good by the most we can in one iteration, we have $\demand[\good]^{t+1} \leq e^{-\frac{1}{5}} \demand[\good]^t$.

Let $c$ be the upper bound on the number of iterations with maximal decreases to the demand of all goods other than $\good$ in order to get a demand of less than 1 for all such goods, we have:
\begin{align}
    {e^{- (\frac{1}{5})}}^c \max_{\good \in \goods} \demand[\good]^0 \leq 1 \nonumber \\
    e^{-\frac{c}{5}}\max_{\good \in \goods}\demand[\good]^0 \leq 1 \nonumber \\
    e^{-\frac{c}{5}} \leq \frac{1}{\max_{\good \in \goods} \demand[\good]^0} \nonumber \\
    -\frac{c}{5} \leq -\log\left( \max_{\good \in \goods}\demand[\good]^0\right) \nonumber \\
    k \geq 5\log\left(\max_{\good \in \goods}\demand[\good]^0\right)\label{max-num-iter-2}
\end{align}

Hence, combining the number of iterations given in \Cref{max-num-iter-1} and \Cref{max-num-iter-2}, we obtain a total number of iterations in which the price of good $\good$ decreases by the maximal factor of $e^{-\frac{1}{5}}$ to be 
\begin{align*}
c+k = 5\log\left(\max_{l \in \goods}\demand[l]^0\right) - 5\log\left( \demand[\good]^0 \right) = 5\log\left(\frac{\max_{l \in \goods}\demand[l]^0}{\demand[\good]^0}\right)    
\end{align*}

Since we are dealing with discrete time steps however, the actual upper bound is $5\log\left(\frac{\max_{l \in \goods}\demand[l]^0}{\demand[\good]^0}\right) + 1$, since $5\log\left(\frac{\max_{l \in \goods}\demand[l]^0}{\demand[\good]^0}\right)$ might not be an integer value. Hence, the after $c+k = 5\log\left(\frac{\max_{l \in \goods}\demand[l]^0}{\demand[\good]^0}\right) + 1$ iteration of maximal decreases in the price of good $\good$ by a factor of $e^{- \frac{1}{5}}$, we get a lower bound on the price given by:
\begin{align*}
    \price[\good]^t &\geq {e^{-(\frac{1}{5})}}^{k+c} \price[\good]^0\\ &= e^{-\frac{k+c}{5}}\price[\good]^0\\
    &= e^{-\frac{5\log\left(\frac{\max_{l \in \goods}\demand[l]^0}{\demand[\good]^0}\right)}{5}}\price[\good]^0\\
    &= \frac{e^{-\frac{1}{5}}}{\frac{\max_{l \in \goods}\demand[l]^0}{\demand[\good]^0}}\price[\good]^0\\
    &\geq \frac{\demand[\good]^0}{2\max_{l \in \goods}\demand[l]^0}\price[\good]^0
\end{align*}

Finally, coupling this with \Cref{upper-demand-subs}, i.e.,  the upper bound on the demand of good $\good$ given prices at time $t$, we get an overall upper bound:
\begin{align*}
    \demand[\good]^t &\leq \frac{\sum_{\buyer \in \buyers} \budget[\buyer]}{\frac{\demand[\good]^0}{2\max_{l \in \goods}\demand[l]^0}\price[\good]^0}\\
    &= 2\frac{\max_{l \in \goods}\demand[l]^0}{\demand[\good]^0} \frac{\sum_{\buyer \in \buyers} \budget[\buyer]}{\price[\good]^0}
\end{align*}

\underline{Case 2: The initial demand for good $\good$ is over 1, i.e.,  $\demand[\good]^0 \geq 1$}

When the demand of good $\good$ goods is above 1   the initialization of the t\^atonnement process, the price of good $\good$ is guaranteed to decrease in the next round. It is, however, possible that in the following rounds the increases in the prices of other goods will lead to decreases in the price of good $\good$. As a result, our goal is to 1) upper bound the number of maximal iterations that decrease the demand for all goods under 1, and 2) use this information to calculate how low the price of good $\good$ can get.

That is, we have to make sure to adjust the price of good $\good$, for each iteration during which an increase in prices of other goods leads the demand of good $\good$ to get under 1 one despite its price increasing. This number of iterations corresponds to the constant $c$ we calculated in case 1. Hence, we obtain an lower bound the price of good $\good$ given by:

% To do so, we first find a lower bound to the decrease in the demand of other goods when their prices are increased, we then use this information to calculate an upper bound on the number of such iterations. Finally, we multiply this iteration number with the maximum decrease in price possible per iteration to obtain the factor by most $\price[\good]^0$ can decrease throughout the algorithm. 

% First, note that the demand obtained by increasing the prices of all goods is a lower bound to the maximum amount by which the demand of can decrease in one iteration since we are in a gross substitutes market. That is, when increasing the price of one good by the most we can in one iteration, we have $\demand[\good]^{t+1} \leq e^{-\frac{1}{5}} \demand[\good]^t$.

% Let $k$ be the upper bound on the number of iterations with maximal decreases to the demand of all goods other than $\good$ in order to get a demand of less than 1 for all such goods, we have:

% \begin{align}
%     {e^{- \frac{1}{5}}}^k \max_{k \in \goods} \demand[k]^0 \leq 1\\
%     e^{-\frac{k}{5}}\max_{k \in \goods}\demand[k]^0 \leq 1\\
%     e^{-\frac{k}{5}} \leq \frac{1}{\max_{k \in \goods} \demand[k]^0}\\
%     -\frac{k}{5} \leq -\log\left( \max_{k \in \goods}\demand[k]^0\right)\\
%     k \geq 5\log\left(\max_{k \in \goods}\demand[k]^0\right)
% \end{align}

% Hence, we have an upper bound of
$5\log\left(\max_{k \in \goods}\demand[k]^0\right)$ on the number of iterations. Since we are in the discrete update case, the upper bound is in reality $5\log\left(\max_{k \in \goods}\demand[k]^0\right)$. This means that we can have at most $5\log\left(\max_{k \in \goods}\demand[k]^0\right)$ rounds of the algorithm during which the demand of good $\good$ stays above one and its price decreases.

Hence, the lowest the price of good $\good$ can get to is:
\begin{align*}
    \price[\good]^t &\geq (e^{-\frac{1}{5}})^{k} \price[\good]^0\\
    &= e^{-\frac{k}{5}} \price[\good]^0\\
    &= e^{-\frac{5\log\left(\max_{k \in \goods}\demand[k]^0\right) + 1}{5}} \price[\good]^0\\
    &= \frac{e^{-\frac{1}{5}}}{\max_{k \in \goods}\demand[k]^0} \price[\good]^0\\
    &\geq \frac{\price[\good]^0}{2\max_{k \in \goods}\demand[k]^0} 
\end{align*}

Combining all of these results, we get an upper bound on the demand throughout the algorithm given by:
\begin{align*}
    \demand[\good]^t &\leq \frac{\sum_{\buyer \in \buyers} \budget[\buyer]}{ \frac{\price[\good]^0}{2\max_{k \in \goods}\demand[k]^0} }\\
    &= 2\max_{k \in \goods}\demand[k]^0\frac{\sum_{\buyer \in \buyers} \budget[\buyer]}{\price[\good]^0}
\end{align*}

To summarize, we have an overall bound given by:
\begin{align*}
    \demand[\good]^0 &\leq \max \left\{2\max_{k \in \goods}\demand[k]^0\frac{\sum_{\buyer \in \buyers} \budget[\buyer]}{\price[\good]^0},  2\frac{\max_{l \in \goods}\demand[l]^0}{\demand[\good]^0} \frac{\sum_{\buyer \in \buyers} \budget[\buyer]}{\price[\good]^0}\right\}\\
    &=2 \frac{\sum_{\buyer \in \buyers} \budget[\buyer]}{\price[\good]^0} \max \left\{\max_{k \in \goods}\demand[k]^0,  \frac{\max_{l \in \goods}\demand[l]^0}{\demand[\good]^0} \right\}\\
\end{align*}
\end{proof}

Finally, we use the upper bounds found on the demand of any good in gross complements CCH and gross substitutes CCH Fisher markets in \Cref{demand-ub-gc} and  \Cref{demand-ub-gs} respectively, we obtain an upper bound on the demand of any good in any CCH Fisher markets (\Cref{upper-bound-demand}).

\upperbounddemand*
\begin{proof}[\Cref{upper-bound-demand}]
Given a fisher market $\calM = (\util, \budget, \ones[\numgoods])$ where $\ones[\numgoods]$ is the supply of each good, fix a good $\good$ and partition the other goods into two sets, a set $S$ which contains goods that are gross substitutes for $\good$ and a set $C$ which contains goods that are complements to $\good$. The sets of goods $S^\good = \{ \good \} \cup S$ and $C^\good = \{ \good \} \cup C$, form bases for respectively a gross substitutes and gross complements markets. We can then create two markets: a gross substitutes CCH Fisher market $\calM_S = (\util, \budget, \s^S)$ where we set the supply vector such that $s_{i}^S = \left\{ \begin{array}{cc}
    1 & \text{if } i \in S^\good \\
    0 & \text{Otherwise} 
\end{array} \right.$, and a gross complements CCH Fisher market $\calM_c = (\util, \budget, \s^{C})$ where we set the supply vector such that $s_{i}^C = \left\{ \begin{array}{cc}
    1 & \text{if } i \in C^\good \\
    0 & \text{Otherwise} 
\end{array} \right.$.

That is, we create from our original market two disjoint gross substitutes and gross complements markets. The highest that the demand for good $\good$ can reach throughout the t\^atonnement process in both markets is respectively $2 \frac{\sum_{\buyer \in \buyers} \budget[\buyer]}{\price[\good]^0} \max \left\{\max_{k \in \goods}\demand[k]^0,  \frac{\max_{l \in \goods}\demand[l]^0}{\demand[\good]^0} \right\}$ and  $2 \max_{k \in \goods} \frac{\demand[\good]^0}{  \demand[k]^0}$. Hence, in our original market the demand of good $\good$ can be at most $2 \frac{\sum_{\buyer \in \buyers} \budget[\buyer]}{\price[\good]^0} \max \left\{\max_{k \in \goods}\demand[k]^0,  \frac{\max_{l \in \goods}\demand[l]^0}{\demand[\good]^0} \right\} + 2 \max_{k \in \goods} \frac{\demand[\good]^0}{  \demand[k]^0}$ since this is the maximum amount by which the demand of good $\good$ can be pushed up by both goods that are gross substitutes and gross complements to it. 
\end{proof}
