# Supplementary material for: A Consumer-Theoretic Characterization of Fisher Market Equilibria
Source: arXiv:2107.08153 source file (2022-01-04)
Supplement: Supplementary file 6 [file proofs_sec5_old.tex]

\begin{proof}[Proof of \cref{continuous-tatonnement-convergence}]
We know that the distance between the t\^atonnement process and the equilibrium price vector can be evaluated using the potential function $\potential$.
Hence, we define $v(t) = \potential(\flow[t](\price))$ to evaluate this distance at time $t$.
Taking the derivative of this function using the chain rule, we obtain:
%
\begin{align}
    \frac{dv}{dt} &= \grad[\price] \potential(\flow[t](\price)) \cdot \frac{d\flow}{dt} \\
    &= \grad[\price] \potential(\flow[t](\price)) \cdot -\grad[\price] \potential(\flow[t](\price)) \\
    &= - ||\grad[\price] \potential(\flow[t](\price)||_2^2 \\
    &= - ||\excess(\flow[t](\price))||_2^2
\end{align}

\noindent
We can now re-express the the potential along the trajectory $v$ as an integral equation:
%
\begin{align}
    v(t) &= v(0) + \int_0^t   - ||\excess(\flow[t](\price))||_2^2\\
    &= v(0) - \int_0^t  ||\excess(\flow[t](\price))||_2^2
\end{align}

\noindent
Note that $||\excess(\price(t))||_2^2 > 0$, unless $\price(t) = \price^*$.
Hence, for any time $t>0$, we have $v(t) \leq v(0)$,
with equality iff the process reaches equilibrium.
Since $\potential$ is strictly convex and its minimum exists, we must then have $\lim_{t \to \infty} \flow[t](\price) = \price^*$.
\end{proof}
